# Supplementary material for: CStream: Parallel Data Stream Compression on Multicore Edge Devices
Source: arXiv:2306.10228 source file (2023-06-25)
Supplement: Supplementary file 1 [file appendix.tex]

% \newpage
% \section{Appendix}
% \label{sec:appendix}
% Due to space limitation, we show the detailed algorithm implementation of tdic32 and lz4 as follows.

% \begin{algorithm}[ht]
% \caption{tdic32 algorithm}
% \label{alg:tdic32}
% \scriptsize
% \LinesNumbered 
% \KwIn{input array $inData$}
% \KwIn{hash table $tb$ with $2^{n}$ entries}
% \KwOut{output array $outData$}
% \While{not reach the end of $inData$} {
% \tcc{(s0) read input data}
%   $number \leftarrow read \ next \ 32-bit from inData$ \label{algo:tdic32_read}\;
% \tcc{(s1) encode data to the tdic32-specific \emph{compact form}}
% $index \leftarrow$ calculate hash value of $number$ \label{algo:tdic32_encode}\;
% $result \leftarrow $ $tb$ [$index$]\;
% \eIf{  $result.word = number$}
% {
   
%     $encoded \leftarrow$  ($index$<<1|1) \; 
%     $bits \leftarrow$ ($n$+1) \;
% }
% {
%     $encoded \leftarrow$  ($number$<<0|1) \;
%     $bits \leftarrow$ (33) \;
%     $tb$ [$index$].$word$ $\leftarrow$ $number$ \label{algo:tdic32_encodeEnd}\;
% }
%   \tcc{(s2) write output data}
%     write ($bits$)-bit $encoded$ to $outData$ \label{algo:tdic32_write}\;
% }
% \end{algorithm}

% \begin{algorithm}[ht]
% \caption{lz4 algorithm}
% \label{alg:lz4}
% \scriptsize
% \LinesNumbered 
% \KwIn{input array $inData$}
% \KwIn{hash table $tb$}
% \KwIn{maximum searching length $ml$}
% \KwOut{output array $outData$}
% $bytePointer\leftarrow$ 0\;
% $literal\leftarrow []$ \;
% \tcp{initially empty array}
% \While{$bytePointer$< $inData.bytes$}
% {   \tcc{(s0) read input data}
%     $number\leftarrow$ read next 32-bit from $inData$, starting from $bytePointer$ \label{algo:lz4_read}\;
%     \tcc{(s1) encode data to the lz4-specific \emph{compact form}}
    
%     $index \leftarrow$ calculate hash value of $number$ {\label{algo:lz4_encode}} \;
%     $result \leftarrow $ $tb$ [$index$]\;
%     $tb[index].offset\leftarrow$ $bytePointer$ \;
%     $tb[index].word\leftarrow$ $number$ \;
%     \If{$bytePointer$>=$inData.bytes$-5}
%     {
%         $literal\leftarrow$ remain part of $inData$  \;
%         goto Line \ref{algo:lz4_write} \;
%     }
%     \eIf{$result.word$=$number$ and $bytePointer-result.offset$ < $ml$}
%     {
%         expand searching and get the $matchLength$\;
%         goto Line \ref{algo:lz4_write} \;
%     }
%     { 
%       append 8-bit $inData[bytePointer]$ to $literal$ \;
%       $bytePointer \leftarrow bytePointer+1$ \label{algo:lz4_encodeEnd}\;
%       goto Line \ref{algo:lz4_read} \;
%     }
%    \tcc{(s2) write output data}
%     encode the \emph{lz4-Token} to $outData$ by $matchLength$ and $literal$ \label{algo:lz4_write}\;
%     $literal\leftarrow []$ \;
%     update $bytePointer$ accordingly\;
%     %\tcp{there is no matching at the end}
% }
% \end{algorithm}


% \subsection{Compression Implementation}
% \label{subsec:compression_implement}
% We use a unified C++ codebase to implemented the listed algorithms in Table~\ref{tab:algo_list}. All stateless stream compression follows the 3-step pattern in Algorithm~\ref{alg:stateless}, and all stateful stream compression follows the 5-step-pattern in Algorithm~\ref{alg:stateful}. By default,
% we use the lazy approach of $s0$ which agglomerates 400 bytes in each micro-batch, and
% the state in all stateful compression is separated (Please refer to Section~\ref{subsec:intro_state}).  

% The implementation of each algorithm follows an incremental relationship as shown in Figure~\ref{fig:algos_evo}.
% Therefore, \emph{we can choose each pair of two arrow-connected algorithms to study algorithm classifications one by one}. First, we directly follow the Android's way~\cite{comp_leb128} in implementing the LEB128, as start point of stateless and byte-aligned stream compression. Second, we adapt byte-unaligned outputting in LEB128 by simplifying the Elias encoding~\cite{comp_elias} as Tcomp32. Specifically, leading zeros of each 32-bit in each tuple is cut off, and the non-zero length in 32 bits is calculated as the prefix. Third, we consider align more bytes by changing LEB128 into Simple8b, by following~\cite{comp_simple8b}. Fourth, we add incremental state to 
% Tcomp32 and LEB128 and construct the Tdic32 and Delta-LEB128, respectively. The tdic32 has a relatively complicated state, which is a lz4-like hash table~\cite{comp_lz4} to record the duplication (4096 table entries by default), and each 32-bit in each tuple may be replaced by its hash index (always shorter than 32-bit) if it has appeared before as recorded by the table. The Delta-LEB128 on the other hand,  maintains a simpler state: it calculate the difference between two consecutive values as the ``delta'' state~\cite{comp_tersecades,comp_baseDelta}, and then use LEB128's approach to output the ``delta'' state instead of original value. In the end, we allow some loss in encoding the ``delta'' state of Delta-LEB128, and construct the adaptive differential pulse-code modulation (ADPCM). Specifically. we use the lossy non-uniform quantization~\cite{comp_nonuniform} in ADPCM to encode the ``delta'' state, instead of the lossless LEB128-style. 
